# Supplementary material for: On the Efficiency of ERM in Feature Learning
Source: arXiv:2411.12029 source file (2024-11-18)
Supplement: Supplementary file 1 [file cor_4.tex]

By the moment assumption, we have that the conclusions of Corollary \ref{cor:2} hold. Now for the first statement, note that if all empirical risk minimizers are in
