# Supplementary material for: On the Efficiency of ERM in Feature Learning
Source: arXiv:2411.12029 source file (2024-11-18)
Supplement: Supplementary file 2 [file prop_1.tex]

Define
\begin{equation*}
    \deltamin \defeq \min_{t \in \mathcal{T} \setminus \mathcal{T}_{*}} R(t, w_{*}(t)) - R_{*}
\end{equation*}
The moment assumptions of the current theorem are sufficient for the weak law of large numbers to hold pointwise for the processes in (\ref{eq:proc_1}) and (\ref{eq:proc_2}). Since the set is finite, a simple union bound shows that it also holds uniformly over $\mathcal{T}$.
The first statement of Theorem \ref{thm:3} then yields
\begin{equation*}
    \Prob\paren*{\hat{t}_{n} \notin \mathcal{T}_{*}} = \Prob\paren*{R(\hat{t}_{n}, w_{*}(\hat{t}_{n})) - R_{*} \geq \deltamin} \to 0 
\end{equation*}
as $n \to \infty$. 

Now let $A_{n}$ denote the event that both $\norm{n^{-1/2}\Lambda_n}_{\infty} < 1$ and $\norm{n^{-1/2}\Delta_{n}(\cdot, t_{*})}_{\infty} < 1$. Clearly $\lim_{n \to \infty} \Prob(A_{n}^{c}) = 0$. Now on this event, we have, combining the two bounds of Lemma \ref{lem:main_lem}, that the rescaled excess risk $n \cdot [R(\hat{t}_{n}, \hat{w}_{n}) - R_{*}]$ is bounded by
\begin{equation}
\label{eq:pf_prop_1_1}
     \frac{1}{2} \cdot \frac{1}{1-\norm{n^{-1/2} \Lambda_{n}}_{\infty}} \cdot \paren*{\frac{1}{1 - \norm{n^{-1/2} \Delta_{n}(\cdot, t_{*})}_{\infty}} + \frac{1}{1-\norm{n^{-1/2} \Lambda_{n}}_{\infty}}} \cdot G^{2}_{n}(\hat{t}_{n}).
\end{equation}
The first three terms converge to $1$ in probability, while we bound the last as follows. Firstly,
\begin{align*}
    \Prob(G_{n}^{2}(\hat{t}_{n}) \geq x) &= \Prob\paren*{\brace{G_{n}^{2}(\hat{t}_{n}) > x} \cap \brace*{\hat{t}_{n} \in \mathcal{T}_{*}}} + \Prob\paren*{\brace{G_{n}^{2}(\hat{t}_{n}) > x} \cap \brace*{\hat{t}_{n} \notin \mathcal{T}_{*}}} \\
    & \leq \Prob\paren*{\max_{s \in \mathcal{T}_{*}} G_{n}^{2}(s) > x}
\end{align*}
